# Supplementary material for: Non-Unitary $3 \times 3$ Mixing in Majorana Neutrinos and Vector-like Quark Models
Source: arXiv:2401.15049 source file (2024-01-26)
Supplement: Supplementary file 1 [file Thesis_Appendix_A.tex]

\chapter{placeholder}
\label{chapter:placeholder}
