# Supplementary material for: Non-Unitary $3 \times 3$ Mixing in Majorana Neutrinos and Vector-like Quark Models
Source: arXiv:2401.15049 source file (2024-01-26)
Supplement: Supplementary file 4 [file Thesis_Appendix_D.tex]

\chapter{Light Neutrino Masses generated at Loop Level in Exact Formalism}
\label{chapter:loopgenerated}
